# Supplementary material for: Impact of octupole deformation on the nuclear electromagnetic response
Source: arXiv:2512.03776 source file (2026-04-23)
Supplement: Supplementary file 1 [file Supplemental-Material.pdf]

# Supplemental Material: Impact of octupole deformation on the nuclear electromagnetic response

Manu Kanerva and Markus Kortelainen

Department of Physics, University of Jyväskylä, P.O. Box 35, FI-40014 Jyväskylä, Finland

(Dated: November 18, 2025)

## I. PHOTOABSORPTION CROSS SECTIONS

Figures 1–5 show photoabsorption cross sections for the Rn, Ra, U, Pu, and Cm isotopic chains with octupole-deformed ground states between mass numbers  $A = 222$ –230 calculated from  $E1$  transition strengths. Additionally, Fig. 6 presents results for very neutron-rich Pu and Cm isotopes. The figures support the observations discussed in the main text. However, it is worth noting that  $^{228}\text{Cm}$  with UNEDF1, as well as very neutron-rich isotopes with SkM\*, exhibit significantly reduced intrinsic quadrupole moments for octupole-deformed HFB solutions compared to the reflection-symmetric ones, as shown in Tab. 1 of the main text. Consequently, the differences between the cross sections of octupole-deformed and reflection-symmetric HFB solutions in these nuclei can largely be attributed to the variation in quadrupole deformation.

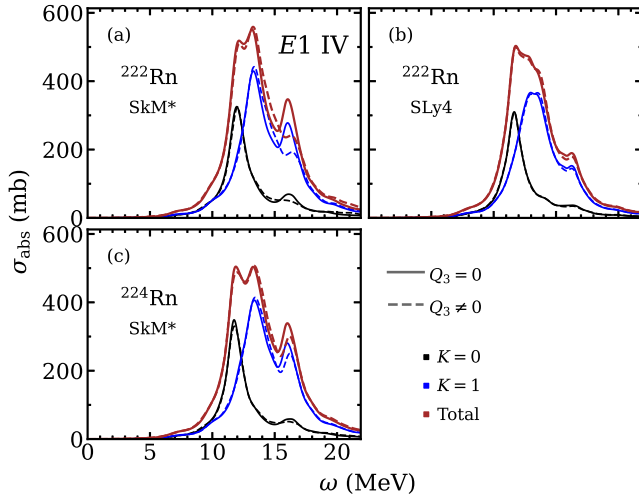

FIG. 1. Photoabsorption cross sections calculated from isovector (IV) electric dipole ( $E1$ ) transition strengths for Rn isotopes. Panels (a)–(c) show results for isotopes with mass numbers  $A = 222$ –224, obtained with those Skyrme energy-density functionals (among SkM\*, SLy4, and UNEDF1) that yield octupole-deformed ground states, as indicated in each subpanel. Solid and dashed lines correspond to reflection-symmetry-conserving ( $Q_3 = 0$ ) and reflection-symmetry-breaking ( $Q_3 \neq 0$ ) HFB ground-state solutions, respectively. The  $K = 1$  mode is shown as the sum of the identical  $K = \pm 1$  modes.

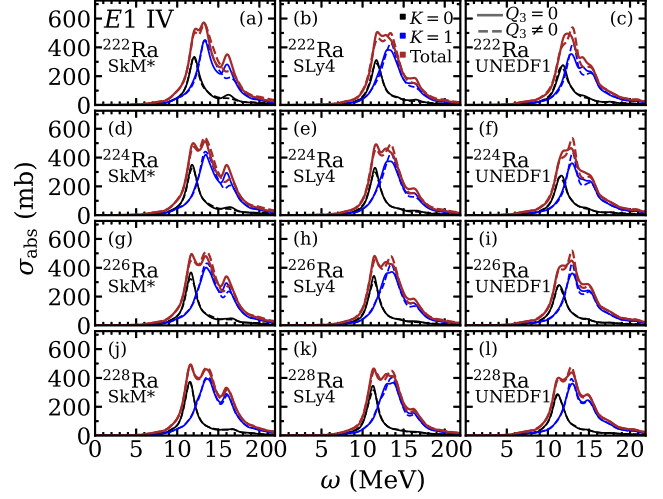

FIG. 2. Same as in Fig. 1, but for Ra isotopes.

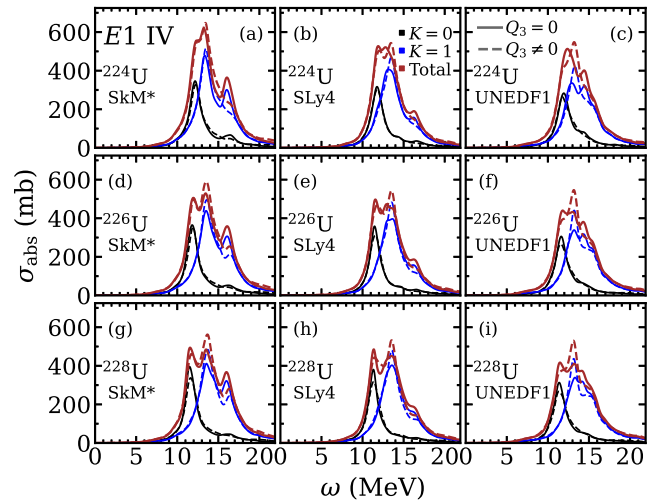

FIG. 3. Same as in Fig. 1, but for U isotopes.

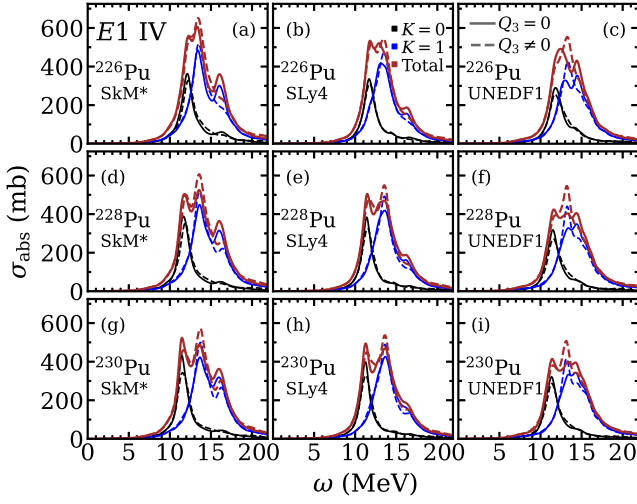

FIG. 4. Same as in Fig. 1, but for Pu isotopes.

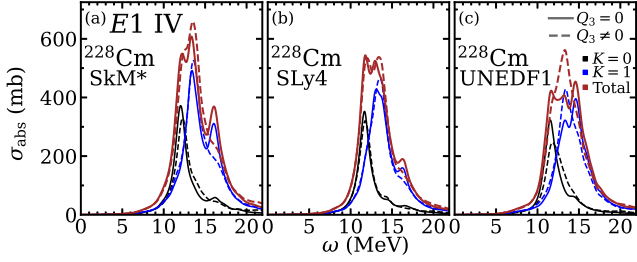

FIG. 5. Same as in Fig. 1, but for  $^{228}\text{Cm}$ .

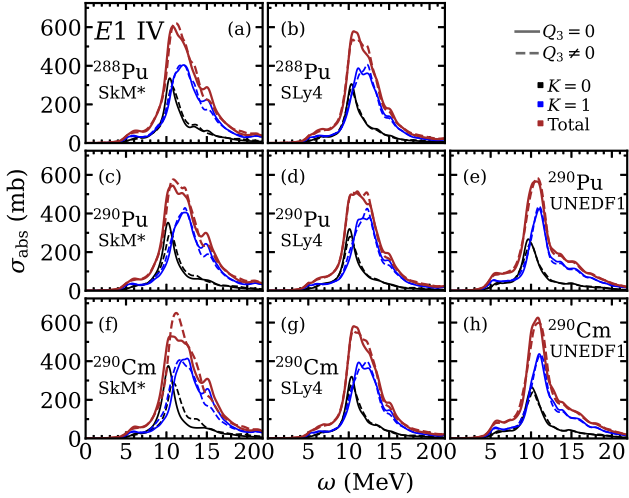

FIG. 6. Same as in Fig. 1, but for very neutron rich  $^{288,290}\text{Pu}$  and  $^{290}\text{Cm}$  isotopes.

## II. M1 TRANSITIONS

Magnetic dipole transition strength functions for Rn, Ra, Th, Pu, and Cm isotopes with  $A = 222-230$ , as well

as for very neutron-rich Pu and Cm isotopes are shown in Figs. 7–12. These figures consistently support the observations discussed in the main text. As in the case of cross sections, variations in quadrupole moments between octupole-deformed and reflection-symmetric HFB solutions in certain isotopes should be taken into account when comparing transition strengths.

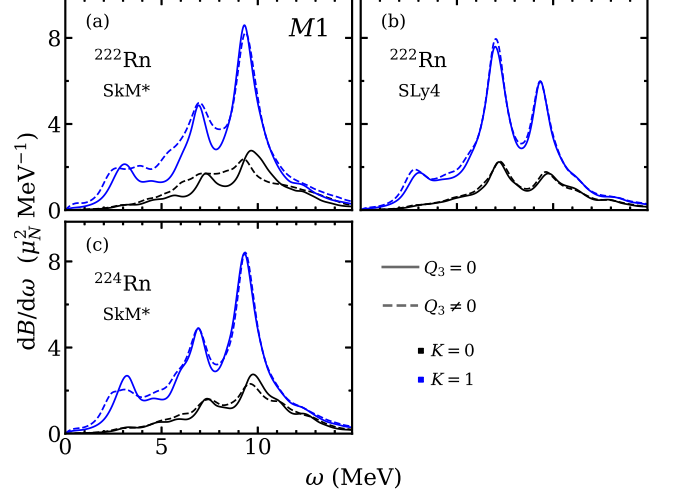

FIG. 7. Magnetic dipole ( $M1$ ) transition strength functions for Rn isotopes. Panels (a)–(c) show results for isotopes with mass numbers  $A = 222-224$ , obtained with those Skyrme energy-density functionals (among SkM\*, SLy4, and UNEDF1) that yield octupole-deformed ground states, as indicated in each subpanel. Solid and dashed lines correspond to reflection-symmetry-conserving ( $Q_3 = 0$ ) and reflection-symmetry-breaking ( $Q_3 \neq 0$ ) HFB ground-state solutions, respectively. Modes with  $K > 0$  are shown as the sum of the corresponding identical positive and negative  $K$  modes.

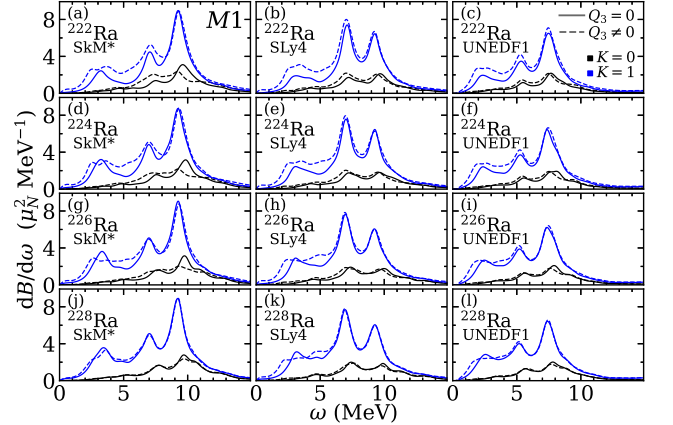

FIG. 8. Same as in Fig. 7, but for Ra isotopes.

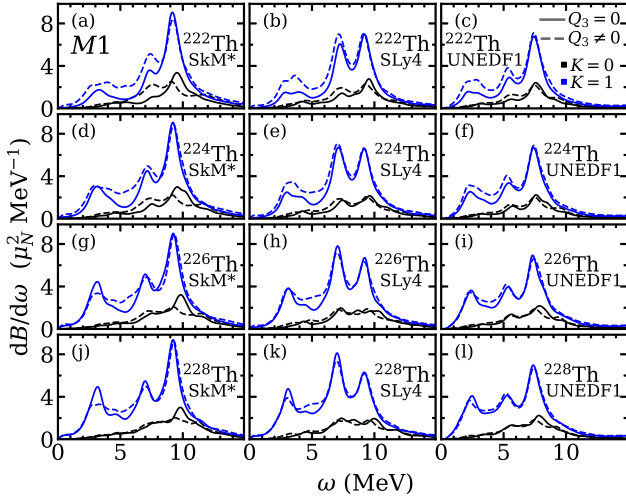

FIG. 9. Same as in Fig. 7, but for Th isotopes.

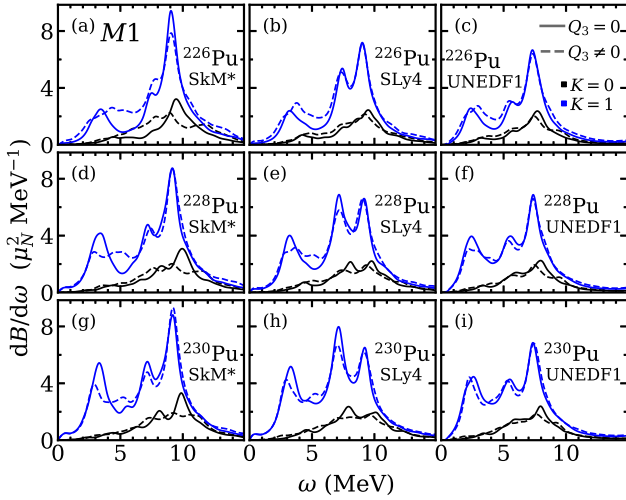

FIG. 10. Same as in Fig. 7, but for Pu isotopes.

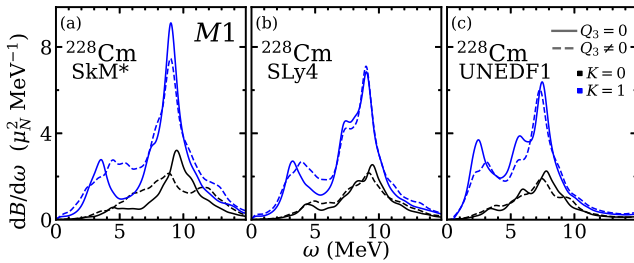

FIG. 11. Same as in Fig. 7, but for  $^{228}\text{Cm}$ .

TABLE I. Fitting parameters  $k$  and  $b$  of the linear fit for the subtracted  $m_0^*$  sum rule in Eq.(1). Details in the text.

|     | SkM* ( $\mu_N^2$ ) | SLy4 ( $\mu_N^2$ ) | UNEDF1 ( $\mu_N^2$ ) |
|-----|--------------------|--------------------|----------------------|
| $k$ | 181.401            | 187.316            | 187.968              |
| $b$ | 2.133              | 2.111              | 3.219.               |

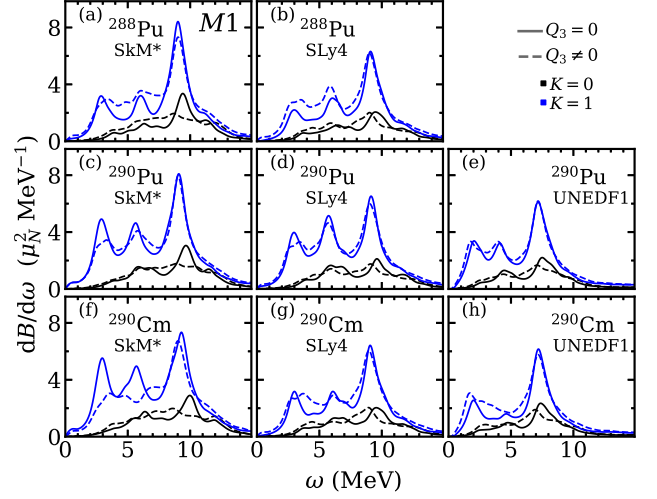

FIG. 12. Same as in Fig. 7, but for very neutron rich  $^{288, 290}\text{Pu}$  and  $^{290}\text{Cm}$  isotopes.

Figure 13 shows the subtracted  $m_0^*$  sum rule of M1 transitions with excitation energies between 0 and 5 MeV for the studied nuclei with mass numbers  $A = 222-230$ , plotted as a function of the octupole moment for octupole-deformed HFB solutions. Here, the subtracted sum rule is defined as

$$m_0^* = m_0 - (k\beta_2^2 + b), \quad (1)$$

where  $m_0$  is the total sum rule, and  $k$  and  $b$  are obtained from the linear fits  $m_0 = k\beta_2^2 + b$ , performed in Figs. 4 (d)–(f) of the main text to the  $Q_3 = 0$  data, with values given in Tab. I. As mentioned in the main text, within this energy range, there is no correlation between the magnitude of octupole deformation and the increase in  $m_0$  for octupole-deformed HFB solutions as shown in Fig. 13.

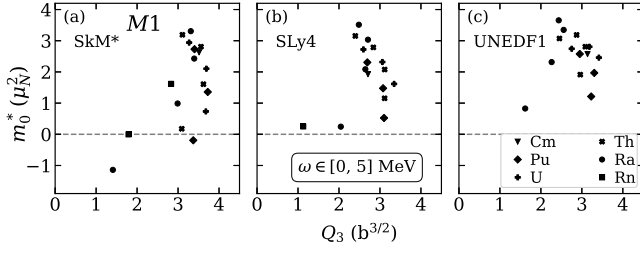

FIG. 13. Subtracted sum rule  $m_0^*$  for magnetic dipole ( $M1$ ) transitions in octupole-deformed HFB solutions of nuclei with  $A = 222-230$ , plotted as a function of the octupole moment  $Q_3$ . Panels show results for (a) SkM\*, (b) SLy4, and (c) UNEDF1 functionals, including transitions with excitation energies between 0 and 5 MeV. Different marker shapes are used to distinguish the isotopic chains.

Figure 14 illustrates that, when considering a narrower energy window around the high-energy scissors mode, the  $m_1$  sum rule values of octupole-deformed HFB solutions are comparable in magnitude to the trend of the reflection-symmetric solutions, as noted in the main text.

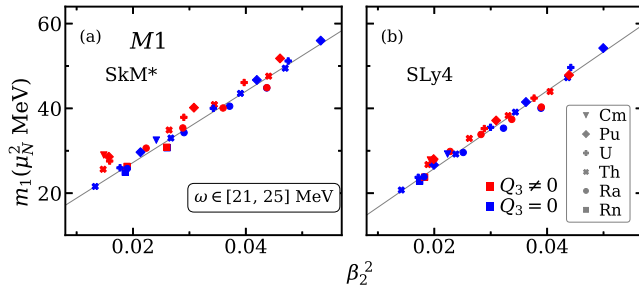

FIG. 14. Energy-weighted sum rules  $m_1$  of magnetic dipole ( $M1$ ) transitions as a function of the square of the quadrupole deformation parameter  $\beta_2$  for the studied nuclei with  $A = 222-230$ . Panels show results for (a) SkM\* and (b) SLy4 functionals, including transitions with excitation energies between 21 and 25 MeV. Blue markers correspond to reflection-symmetry-conserving ( $Q_3 = 0$ ) and red markers to reflection-symmetry-breaking ( $Q_3 \neq 0$ ) HFB ground-state solutions. Marker shapes distinguish isotopic chains. The straight line represents a linear fit to the  $Q_3 = 0$  data.

### III. ISOSCALAR $E2$ TRANSITIONS

Isoscalar electric quadrupole transition strength functions for Rn, Ra, U, Pu, and Cm isotopes with  $A = 222-230$ , as well as for very neutron-rich Pu and Cm isotopes are shown in Figs. 15–20. In these calculations, the spurious rotational contribution from the  $K = 1$  mode has been removed. The results support the observations discussed in the main text. As before, variations in quadrupole moments between octupole-deformed and reflection-symmetric HFB solutions in certain isotopes should be taken into account when comparing transition strengths. However, in contrast to the discussion in the

main text, the resonances are shifted by approximately 1 MeV lower for neutron-rich isotopes as expected due to the change in mass number [1].

At low energies, the transition strength of the  $K = 0$  mode reaches a very high value,  $dB/d\omega \approx 0.30 e^2 b^2 \text{MeV}^{-1}$ , for the reflection-symmetric HFB solution of  $^{228}\text{Cm}$  calculated with UNEDF1, as shown in Fig. 19 (c). This behavior can be attributed to the very soft potential energy surface (PES) in the  $Q_2$  direction of the corresponding HFB solution, as shown in Fig. 21. This observation is consistent with the discussion in the main text regarding the influence of the PES on low-energy transition strengths. Similarly, in Fig. 19 (c), the  $K = 2$  mode – plotted as a sum of  $K = 2$  and  $K = -2$  modes – reaches a very high transition strength close to zero energy, indicating  $\gamma$ -softness at that point of the PES. In addition,  $^{290}\text{Cm}$  calculated with SkM\* in Fig. 20 (f) exhibits a very high value of the summed  $K = 2$  mode transition strength,  $dB/d\omega \approx 0.66 e^2 b^2 \text{MeV}^{-1}$  (truncated in the figure), indicating  $\gamma$ -softness or a saddle point with respect to the  $Q_{22}$  direction at that point of the PES.

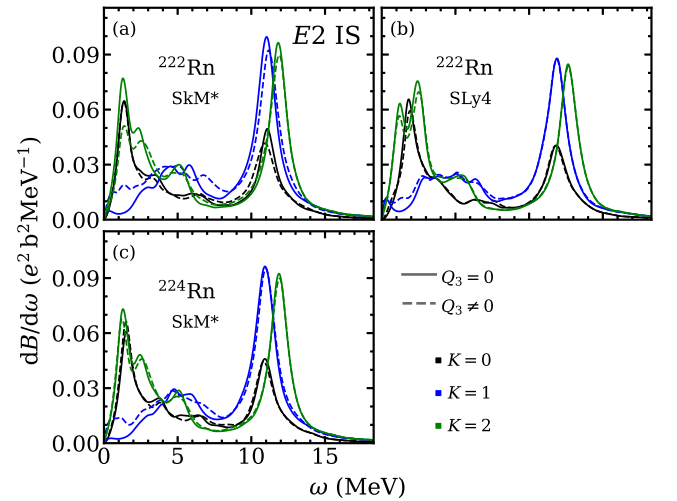

FIG. 15. Same as in Fig. 7, but showing isoscalar (IS) electric quadrupole ( $E2$ ) transitions for Rn isotopes.

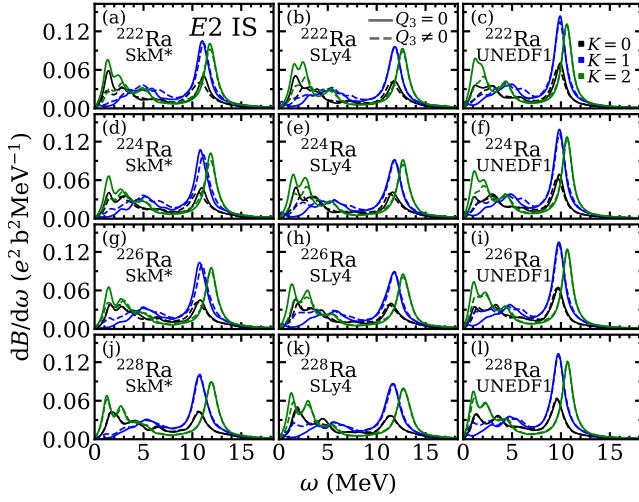

FIG. 16. Same as in Fig. 7, but showing isoscalar (IS) electric quadrupole ( $E2$ ) transitions for Ra isotopes.

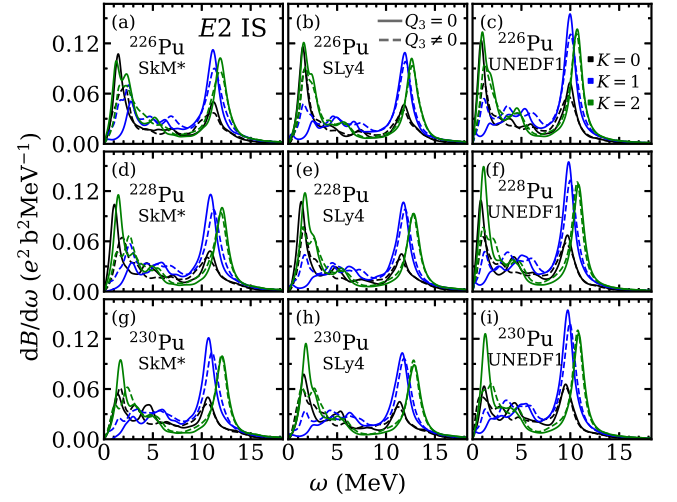

FIG. 18. Same as in Fig. 7, but showing isoscalar (IS) electric quadrupole ( $E2$ ) transitions for Pu isotopes.

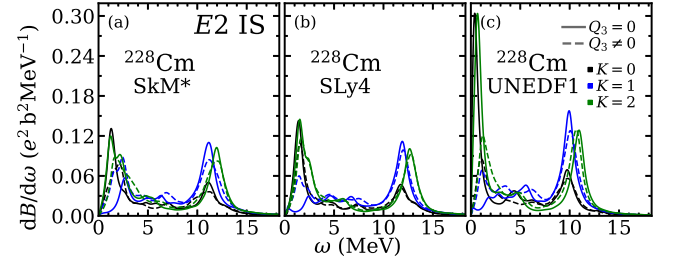

FIG. 19. Same as in Fig. 7, but showing isoscalar (IS) electric quadrupole ( $E2$ ) transitions for  $^{228}\text{Cm}$ .

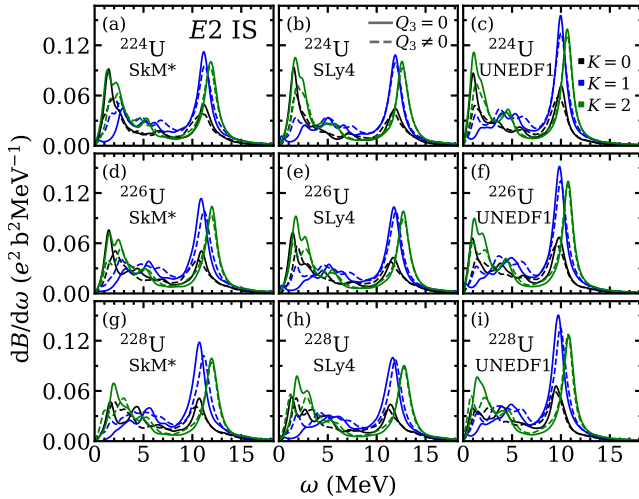

FIG. 17. Same as in Fig. 7, but showing isoscalar (IS) electric quadrupole ( $E2$ ) transitions for U isotopes.

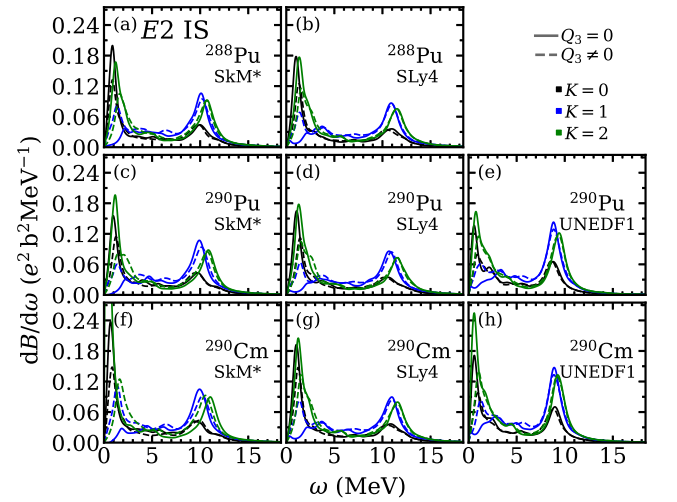

FIG. 20. Same as in Fig. 7, but showing isoscalar (IS) electric quadrupole ( $E2$ ) transitions for very neutron rich  $^{288,290}\text{Pu}$  and  $^{290}\text{Cm}$  isotopes.

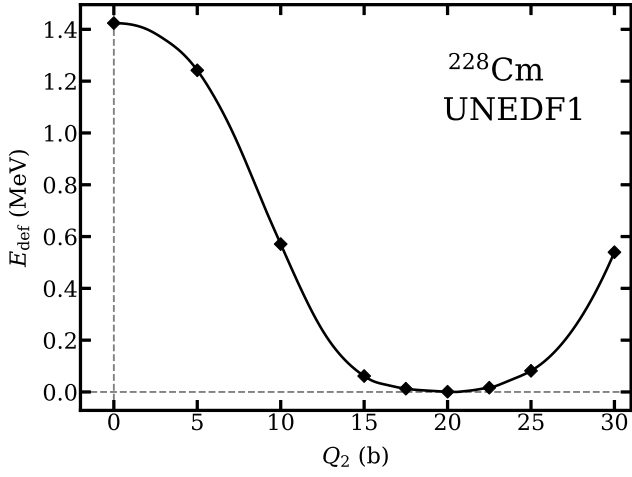

FIG. 21. Deformation energy of  $^{228}\text{Cm}$  as a function of the quadrupole moment  $Q_2$ , for reflection-symmetric HFB solutions calculated with the UNEDF1 functional. The reflection-symmetric HFB ground-state solution occurs at  $Q_2 = 20.438$  b.

#### IV. ISOVECTOR $E2$ TRANSITIONS

Isovector electric quadrupole transition strength functions for Rn, Ra, Th, Pu, and Cm isotopes with  $A = 222 - 230$ , as well as for very neutron-rich Pu and Cm isotopes are shown in Figs. 22–27. These figures consistently support the observations discussed in the main text. As mentioned, variations in quadrupole moments between octupole-deformed and reflection-symmetric HFB solutions in certain isotopes should be taken into account when comparing transition strengths.

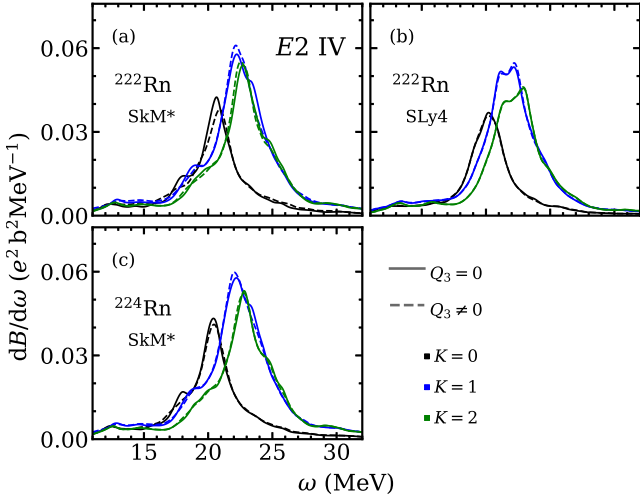

FIG. 22. Same as in Fig. 7, but showing isovector (IV) electric quadrupole ( $E2$ ) transitions for Rn isotopes.

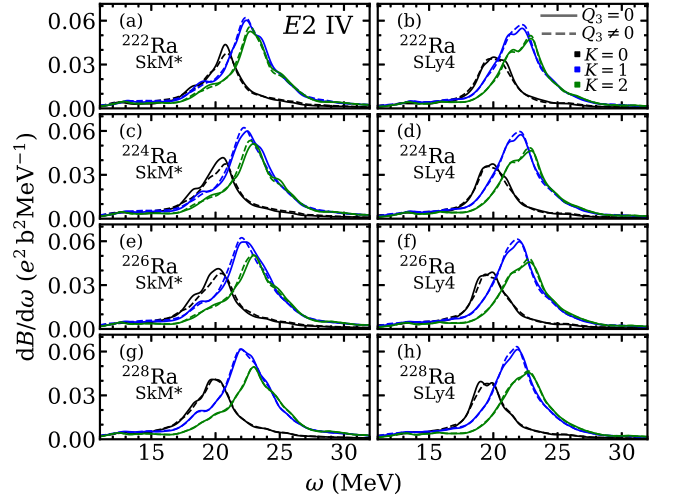

FIG. 23. Same as in Fig. 7, but showing isovector (IV) electric quadrupole ( $E2$ ) transitions for Ra isotopes omitting the UNEDF1 functional.

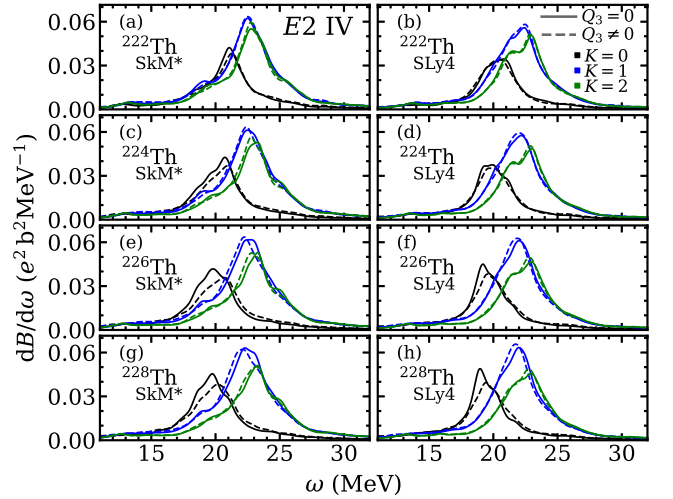

FIG. 24. Same as in Fig. 7, but showing isovector (IV) electric quadrupole ( $E2$ ) transitions for Th isotopes omitting the UNEDF1 functional.

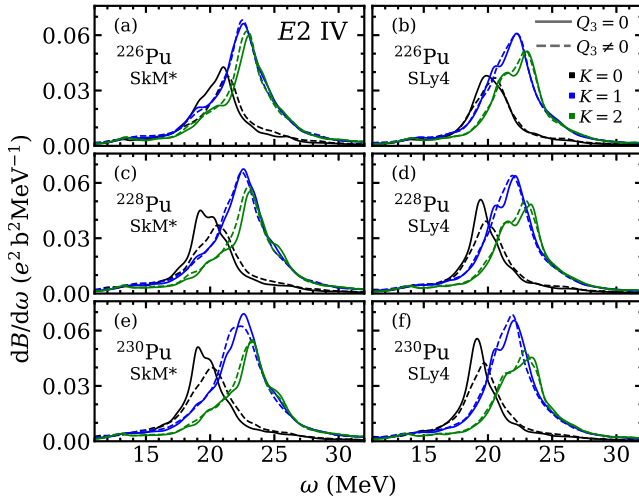

FIG. 25. Same as in Fig. 7, but showing isovector (IV) electric quadrupole ( $E2$ ) transitions for Pu isotopes omitting the UNEDF1 functional.

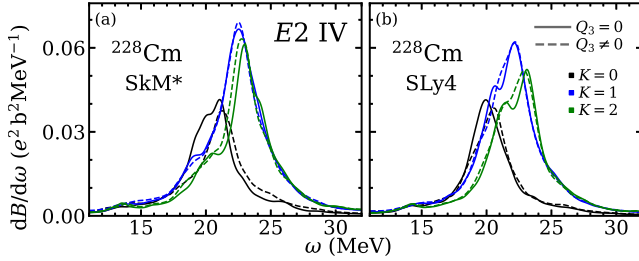

FIG. 26. Same as in Fig. 7, but showing isovector (IV) electric quadrupole ( $E2$ ) transitions for  $^{228}\text{Cm}$  omitting the UNEDF1 functional.

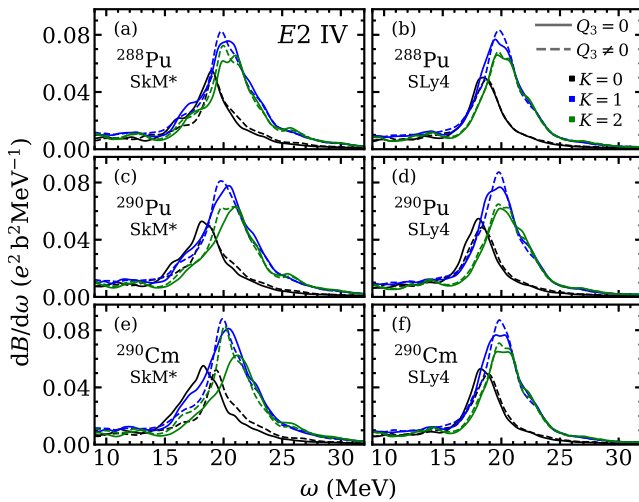

FIG. 27. Same as in Fig. 7, but showing isovector (IV) electric quadrupole ( $E2$ ) transitions for very neutron rich  $^{288,290}\text{Pu}$  and  $^{290}\text{Cm}$  isotopes omitting the UNEDF1 functional.

## V. ISOSCALAR $E3$ TRANSITIONS

Figures 28 and 29 show isoscalar electric octupole transition strength functions for Ra isotopes with  $A = 222\text{--}228$  over a broad energy range and at low excitation energies, respectively. In these calculations, the spurious center-of-mass motion of the  $K = 0$  and  $K = 1$  modes has been removed. In addition, the spurious rotational contribution from the  $K = 1$  mode in octupole-deformed HFB solutions has been removed, as discussed in the main text. As before, variations in quadrupole moments between octupole-deformed and reflection-symmetric HFB solutions in certain isotopes should be considered when comparing transition strengths.

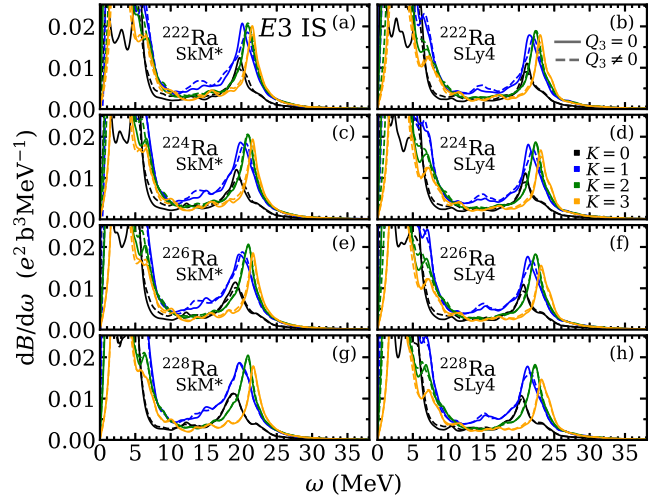

FIG. 28. Same as in Fig. 7, but showing isoscalar (IS) electric octupole ( $E3$ ) transitions for Ra isotopes omitting the UNEDF1 functional.

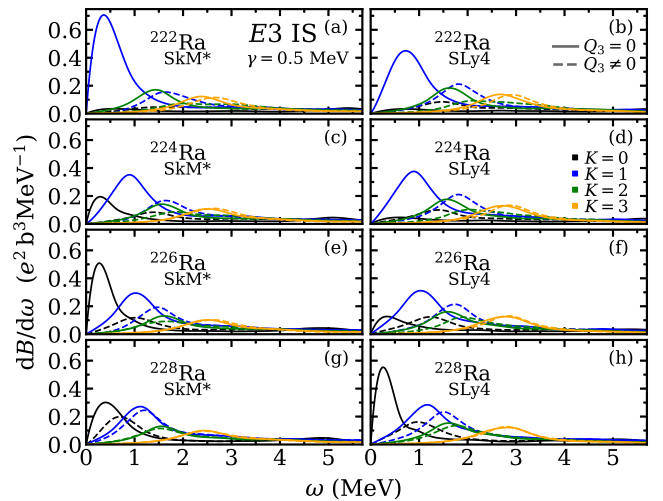

FIG. 29. Same as in Fig. 28, but focusing on lower excitation energies.

## VI. ISOVECTOR $E3$ TRANSITIONS

Figures 30–35 show isovector electric octupole transition strength functions for Rn, Ra, Th, Pu, and Cm isotopes with  $A = 222–230$ , as well as for very neutron-rich Pu and Cm isotopes. Only Ra isotopes were calculated for both reflection-symmetric and reflection-symmetry-breaking HFB solutions, while the remaining isotopes were computed only for the octupole-deformed solution. In all calculations, the spurious center-of-mass motion of the  $K = 0$  and  $K = 1$  modes has been removed. As before, variations in quadrupole moments between octupole-deformed and reflection-symmetric HFB solutions in certain isotopes should be considered when comparing transition strengths.

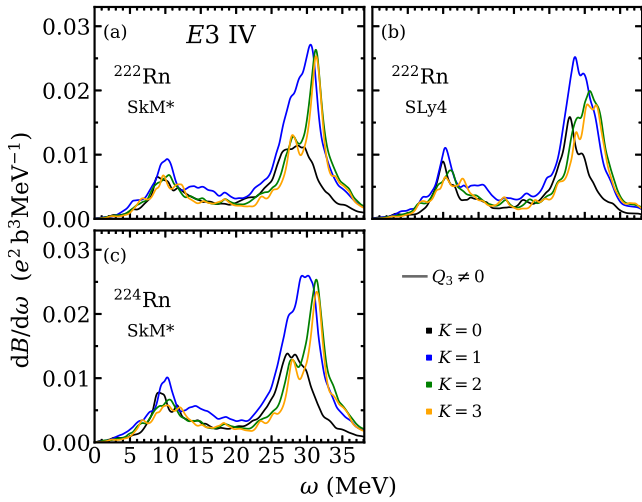

FIG. 30. Same as in Fig. 7, but showing isovector (IV) electric octupole ( $E3$ ) transitions for Rn isotopes – only for the reflection-symmetry-breaking ( $Q_3 \neq 0$ ) HFB solution (solid line), with the UNEDF1 functional omitted.

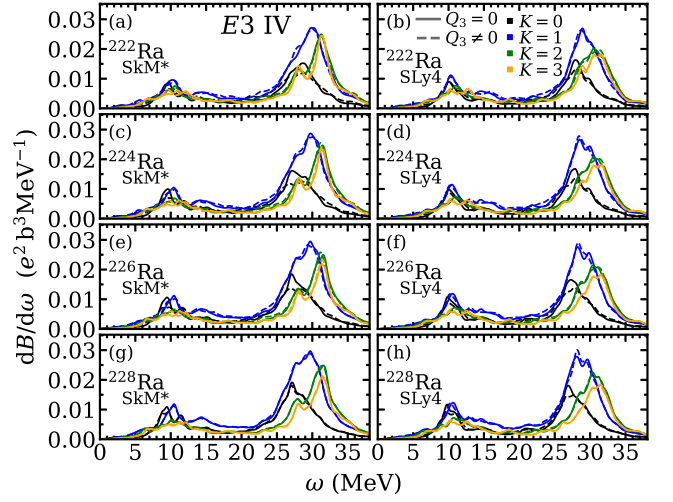

FIG. 31. Same as in Fig. 7, but showing isovector (IV) electric octupole ( $E3$ ) transitions for Ra isotopes omitting the UNEDF1 functional.

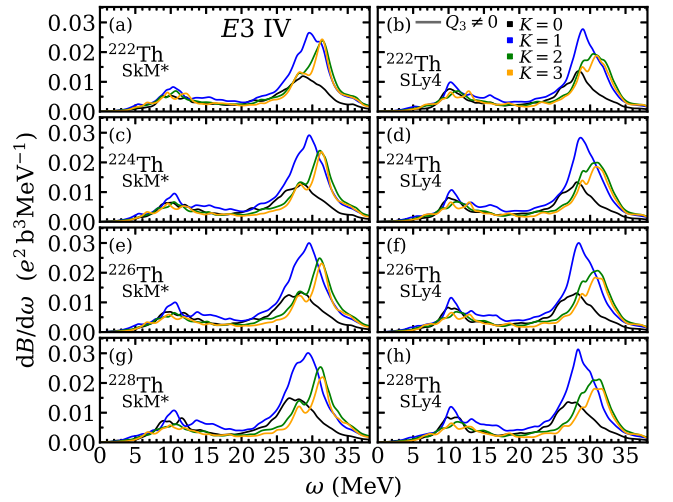

FIG. 32. Same as in Fig. 7, but showing isovector (IV) electric octupole ( $E3$ ) transitions for Th isotopes – only for the reflection-symmetry-breaking ( $Q_3 \neq 0$ ) HFB solution (solid line), with the UNEDF1 functional omitted.

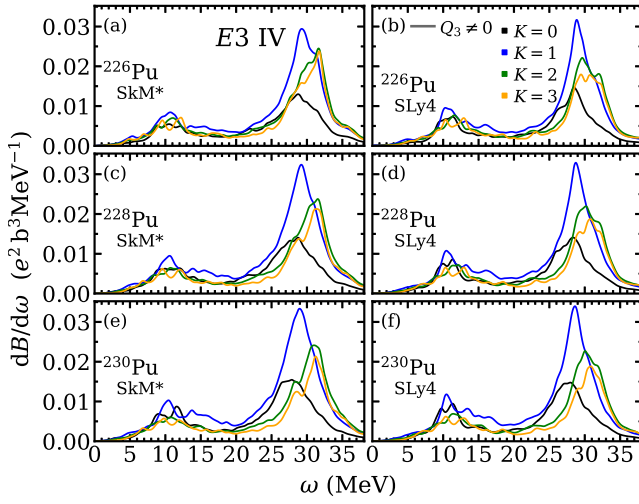

FIG. 33. Same as in Fig. 7, but showing isovector (IV) electric octupole ( $E3$ ) transitions for Pu isotopes – only for the reflection-symmetry-breaking ( $Q_3 \neq 0$ ) HFB solution (solid line), with the UNEDF1 functional omitted.

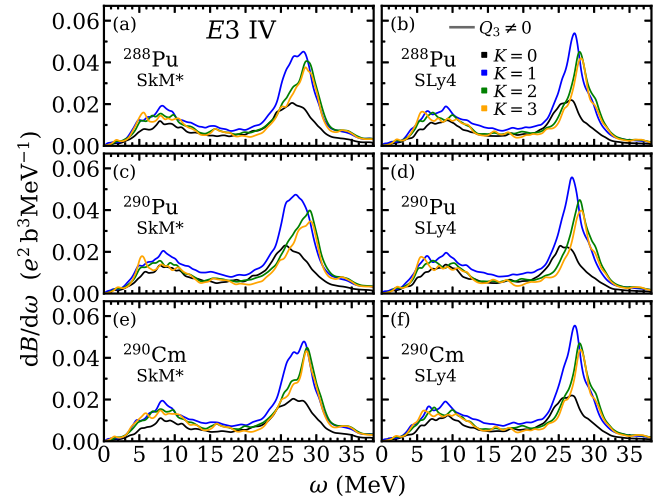

FIG. 35. Same as in Fig. 7, but showing isovector (IV) electric octupole ( $E3$ ) transitions for very neutron rich  $^{288,290}\text{Pu}$  and  $^{290}\text{Cm}$  isotopes – only for the reflection-symmetry-breaking ( $Q_3 \neq 0$ ) HFB solution (solid line), with the UNEDF1 functional omitted.

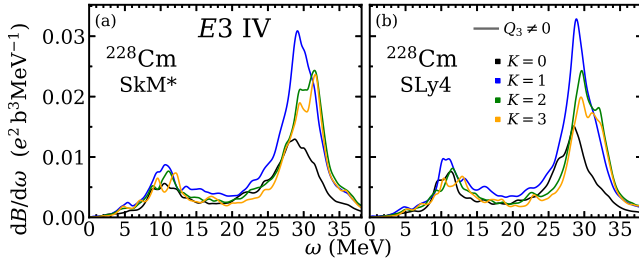

FIG. 34. Same as in Fig. 7, but showing isovector (IV) electric octupole ( $E3$ ) transitions for  $^{228}\text{Cm}$  – only for the reflection-symmetry-breaking ( $Q_3 \neq 0$ ) HFB solution (solid line), with the UNEDF1 functional omitted.

- 
- [1] G. Scamps and D. Lacroix, Systematics of isovector and isoscalar giant quadrupole resonances in normal and superfluid spherical nuclei, [Phys. Rev. C \*\*88\*\*, 044310 \(2013\)](#).
